# Supplementary material for: DeUEDroid: Detecting Underground Economy Apps Based on UTG Similarity
Source: arXiv:2209.01317 source file (2024-11-18)
Supplement: Supplementary file 1 [file appendix.tex]

\appendix
\begin{appendices}
\section{Network Imprint}
\label{appendix}
Figure~\ref{fig:token} presents an example of our network imprint generation process. Initially, the program loads specific APIs (\eg, WebView.loadURL()) and conducts a backward taint analysis to examine the network imprints. The detailed methodology is outlined in Section~\ref{subsec:gui_identify}.

\begin{figure}[H]
\centering
	\includegraphics[width=.45\textwidth]{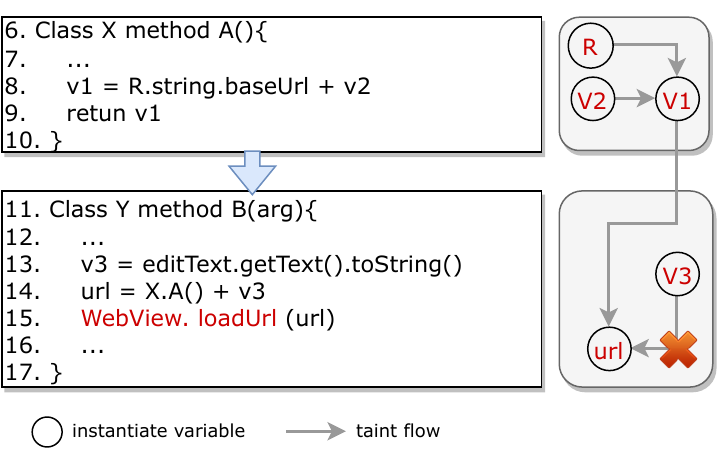}
	\caption{The example of network imprint generation.}
	\label{fig:token}
\end{figure} 

\section{Time Consumption}
Figure~\ref{fig:time} shows the average time consumption for different app sizes. The time consumption for \system{} remains stable, with a fluctuation of merely 67 seconds in the range of 15M-57M. This demonstrates that our system is resilient to large sizes. The detailed experimental methodology is described in Section~\ref{subsubsec:rq3}.

\begin{figure}[H]
\centering
	\includegraphics[width=0.45\textwidth]{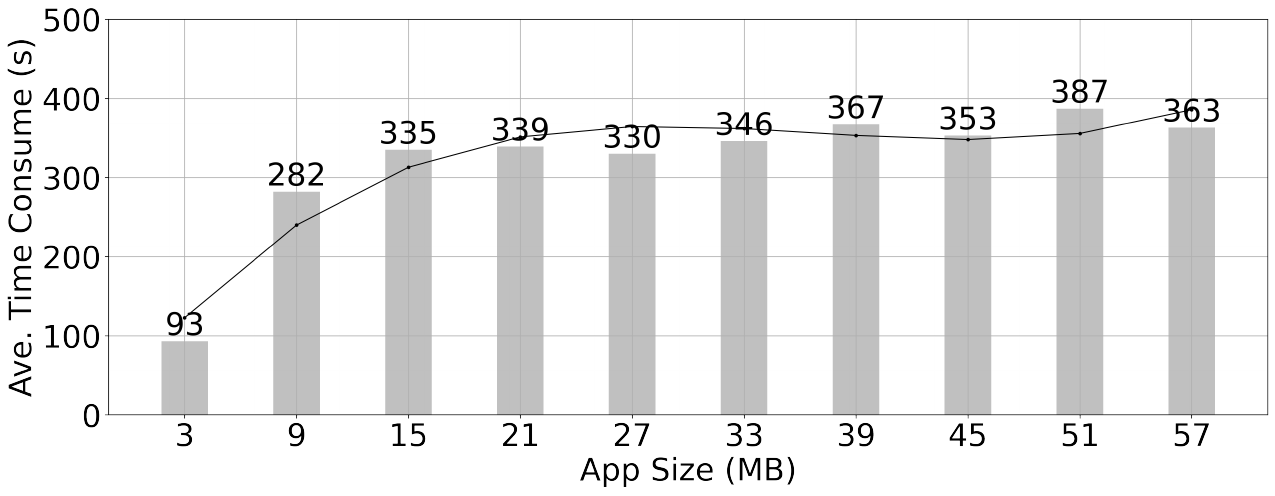}
	\caption{Time consumption distribution.}
	\label{fig:time}
\end{figure}
\end{appendices}

\newpage
